# Supplementary material for: On the Throughput/Bit-Cost Tradeoff in CSMA Based Cooperative Networks
Source: arXiv:0906.1189 source file (2009-11-04)
Supplement: Supplementary file 1 [file appendix.tex]

\appendix

\newcommand{\entspricht}{\mathrel{\widehat{=}}}
Note that $K_m \entspricht$ number of consecutive heads a sequence starts with
that has been generated by tossing a fair coin $m$ times. Define $\mu\coloneqq\mathrm{E}[X]=1/2$ and $\bar{X}_m = \frac{1}{m} \sum_{i=1}^m X_i$. We then have
\begin{align}
P\left[|\bar{X}_m-\mu|<\epsilon,\frac{K_m}{m}<\epsilon\right]
&\geq P\left[|\bar{X}_m-\mu|<\epsilon,\frac{K_m}{m}<\frac{\epsilon}{2}\right]\\
&=P\left[|\bar{X}_m-\mu|<\epsilon\,\Big\vert\,\frac{K_m}{m}<\frac{\epsilon}{2}\right
]P\left[\frac{K_m}{m}<\frac{\epsilon}{2}\right]\label{eq:factors}
\end{align}
First factor in \eqref{eq:factors}:
\begin{align}
P\left[|\bar{X}_m-\mu|<\epsilon\,\Big\vert\,\frac{K_m}{m}<\frac{\epsilon}{2}\right
]
&=P\Bigl[\underbrace{\bar{X}_m-\mu}_{\text{max. for }
K_m=\frac{\epsilon m}{2}}<\epsilon,\underbrace{\mu-\bar{X}_m}_{\text{min. for}
K_m = 0} <\epsilon\, \Big\vert\, \frac{ K_m }{ m } <\frac{\epsilon}{2}
\Bigr]\\
&\geq P\left[\frac{\sum_{i=1}^{m-\frac{\epsilon m}{2}}
X_i+\frac{\epsilon m}{2}}{m}-\mu<\epsilon,\mu-\frac{\sum_{i=1}^{m-1} X_i}{m}
<\epsilon
\right]\\
&\geq P\left[\frac{\sum_{i=1}^{m}
X_i+\frac{\epsilon m}{2}}{m}-\mu<\epsilon,\mu-\frac{\sum_{i=1}^{m} X_i -1}{m}
<\epsilon
\right]\\
&\geq P\left[\frac{\sum_{i=1}^{m}
X_i}{m}-\mu<\frac{\epsilon}{2},\mu-\frac{\sum_{i=1}^{m} X_i}{m}
<\epsilon-\frac{1}{m}
\right]\\
&\geq
P\left[|\bar{X}_m-\mu|<\min\left\{\frac{\epsilon}{2},\epsilon-\frac{1}{m}\right\}
\right ]
\label{eq:firstFactor}
\end{align}
Weak law of large numbers: right hand side of~\eqref{eq:firstFactor} goes to one for
$m\rightarrow\infty$. Second factor in \eqref{eq:factors}:
\begin{align}
P\left[\frac{K_m}{m}<\frac{\epsilon}{2}\right]\geq
P\left[\frac{K_\infty}{m}<\frac{\epsilon}{2}\right]
\geq P\left[K_\infty<\frac{m\epsilon}{2}\right]
= 1-P\left[K_\infty\geq\frac{m\epsilon}{2}\right]
= 1-\left(\frac{1}{2}\right)^\frac{
m\epsilon}{2}.\label{eq:secondFactor}
\end{align}
Obviously, right hand side of \eqref{eq:secondFactor} goes to one for
$m\rightarrow\infty$. Combining \eqref{eq:firstFactor} and
\eqref{eq:secondFactor} shows \eqref{eq:toprove}.
